# Supplementary material for: Inaudible Adversarial Perturbation: Manipulating the Recognition of User Speech in Real Time
Source: arXiv:2308.01040 source file (2023-09-12)
Supplement: Supplementary file 1 [file additional.tex]

%  !TEX root = ../dolphin2.tex

\subsection{Wakeup Authentication Penetration}
The proposed technical approaches can achieve targeted voice command alteration for human-interactive scenarios, however, as for human-absent case, the voice assistant should be woken up first to drive it execute malicious commands. Different from the adversarial examples against ASV~\cite{chen2021fakebob,deng2022fencesitter} which only optimizes the expectation problem of bypassing the ASV, an adversary should satisfy both voiceprint matching and speech recognized as the correct wakeup phrase $Y_w$, such as ``Hey Siri''.
Since the attacker accesses to only 1\textasciitilde3 victim's utterance samples unrelated to the wakeup phrase, we apply the text-to-speech (TTS) tool for synthesizing ``Hey Siri'', meeting the wakeup word recognition requirement firstly. As overlaying adversarial noise to manipulate the voiceprint will also affect the speech recognition,
we consider a joint optimization of speaker embedding similarity (voiceprint loss $\mathcal{L}_{ASV}$) and speech recognition accuracy (CTC loss $\mathcal{L}_{CTC}$) based on above methods. Namely, we aim to find a perturbation $\delta_w$ making the overall voiceprint after superimposing synthesized audio $x_{tts}$ close to the original victim's, it still ensures the wakeup word recognized correctly.
Moreover, we especially splice the perturbation with the beginning or end of the original audio, compared to overlaying it on the audio's middle region, the semantic information is well preserved, and the $\mathcal{L}_{CTC}$ can converge faster from the speech recognition perspective, which greatly reduces the complexity of our optimization as follows:

\begin{equation}
    \delta_{w} = \underset{\delta_w}{\operatorname{argmin}}[\mathcal{L}_{ASV}(x_{tts}+\delta_w, x_{vic}) + \alpha\mathcal{L}_{CTC}(x_{tts}+\delta_w,Y_w)]
\end{equation}
where $L_{ASV}$ is the inverse cosine similarity score between the speaker embedding of $x_{tts}+\delta_w$ and $x_{vic}$ that are extracted by the state-of-the-art speaker verfication model ECAPA-TDNN~\cite{2020ecapatdnn}. We empirically set $\alpha$ to 0.01, which is a hyper-parameter adjusting the weights of two losses.
